# Supplementary material for: Magnetotransport in phase-separated (Ga,Fe)N with $\gamma$'-Ga$_y$Fe$_{4-y}$N nanocrystals
Source: arXiv:1809.08894 ancillary file (2018-09-24)
Supplement: Supplementary file 1 [file Supplemental_Material_AMR.pdf]

# Supplemental Material to: Magnetotransport in phase-separated (Ga,Fe)N with $\gamma$'-$Ga_yFe_{4-y}N$ nanocrystals

September 21, 2018

A. Navarro-Quezada, M. Aiglinger, B. Faina, K. Gas, M. Matzer, Tian Li, R. Adhikari, M. Sawicki and A. Bonanni

## 1 Thermal annealing of Sample A

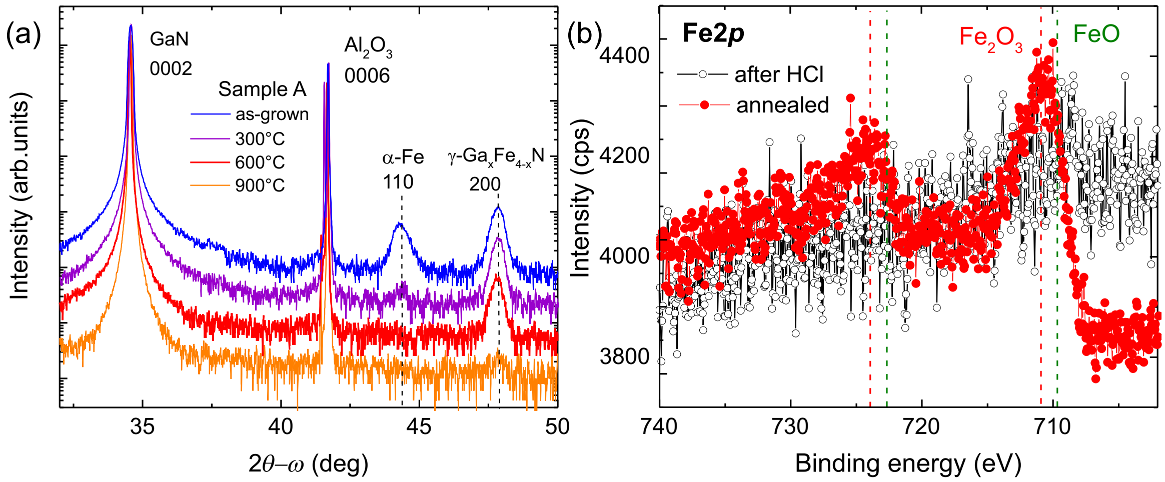


Fig.S 1: (a) HRXRD spectra of Sample A before and after annealing at 300°C, 600°C and 900°C. (b) XPS: Fe2$p$ core level spectra of Sample A annealed to 600°C (Sample A*) before and after a HCl treatment.

The annealing on Sample A at different temperatures confirms the instability of the $\alpha$-Fe nanocrystals (NCs) present upon growth. Already after annealing at 300°C, the (high-resolution) x-ray diffraction (HRXRD) peak originating from the (110) planes of these NCs is significantly reduced, as evidenced in Fig.S 1(a), pointing at the onset of Fe out-diffusion at this temperature. The $FeO_x$ polycrystals formed at the sample surface after the annealing-induced dissolution of $\alpha$-Fe are effectively removed without affecting the sample surface through a chemical treatment of 1 hour in HCl at 37%. This is corroborated by comparing the x-ray photoemission spectroscopy (XPS) spectra of the Fe2$p$ core level peaks presented in Fig. S1(b). The spectrum acquired on the sample after annealing at 600°C shows the Fe2$p$ double peaks at binding energies between 710 eV and 725 eV, indicating the presence of Fe in either the $Fe_2O_3$ or FeO oxidation state at the sample surface. After the HCl treatment, the Fe2$p$ core level peaks are quenched, suggesting the removal of the $Fe_xO$ located at the surface. This is further supported by the fact that the Fe2$p$ spectrum of the as-grown sample (Sample A) resembles the one acquired upon HCl treatment.

## 2 Electrical contacts

In order to ensure the stability of Sample A and Sample A*, the evaporation of metal contacts followed by an annealing has been avoided. The electrical contacts on these samples are prepared according to the following procedure: (i) pressed-on In at each corner of a (5×5) $mm^2$ specimen, (ii) diffusion of In at the surface by local melting with a soldering tip (maximum temperature 300°C) for 10 seconds, (iii) bonding with a 25 $\mu$m gold wire. This procedure has been actually employed on Sample A, on Sample A* and on the GaN reference, resulting in an ohmic behavior down to 2 K. Since Sample B is highly resistive, In could not ensure ohmic contacts,

therefore electron beam/thermal evaporation of Ti, Al, Au stacks has been employed, followed by rapid thermal annealing at 750°C for 30 seconds in nitrogen-rich environment.

## 3 Difference in magnetization between Sample A and Sample A*

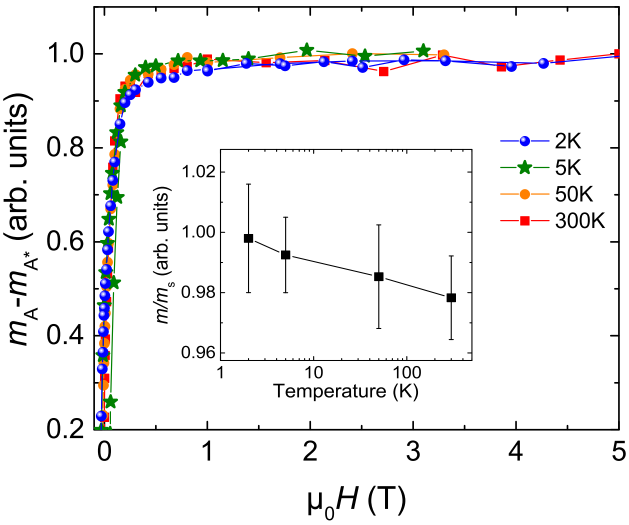


Fig.S 2: The difference in normalized aerial magnetic moment as a function of applied magnetic field between Sample A and Sample A*. Inset: Saturation magnetization of the difference in magnetic moment as a function of $T$.

According to the HRXRD spectra collected in Fig.S 1, no $\alpha$-Fe NCs are present in the Sample A annealed at 600°C, *i.e.* Sample A*. Therefore, the difference $m_{\mathrm{A}}(H,T) - m_{\mathrm{A}*}(H,T)$ in the normalized aerial magnetic moment between Sample A and Sample A* is calculated at each temperature and magnetic field. The dependence on the applied magnetic field is given in Fig.S 2. The difference is nearly temperature independent and saturates swiftly with increasing field, pointing at a firm ferromagnetic component present only in Sample A and originating from $\alpha$-Fe NCs, as confirmed by HRXRD and high-resolution transmission electron microscopy. From the extremely weak dependence of the difference in the magnetic response on temperature, it is inferred that the paramagnetic contribution in both samples is comparable, *i.e.* the annealing – even up to 600°C – does not affect the concentration of the dilute Ga-substitutional Fe ions in the layers. The inset to Fig.S 2 provides the temperature dependence of the magnetization difference in accord with previous observations on an ensemble of Fe nanoparticles [1].

## 4 Magnetoresistance of the GaN reference and Sample B

The magnetoresistance (MR) as a function of applied magnetic field of the unintentionally $n$-type doped GaN reference layer is plotted in Fig.S 3(a) for selected temperatures. Above 50 K the MR is positive, while it is negative below this temperature. The negative MR (NMR) has been analyzed following the procedure reported in Ref. [2] for $n$-InP, where it is claimed that the temperature dependence of the hopping length $R_{\mathrm{h}}$ determines the temperature dependence of the MR. In three-dimensional systems where the Mott variable-range hopping (VRH) regime is observed, $R_{\mathrm{h}} \sim \mathrm{T}^{-1/4}$, leading to a quadratic NMR:

$$\Delta\rho/\rho \approx f_1(H)H^2 \tag{1}$$

with $f_1(H) \sim T^{-3/4}$ [3]. The temperature dependence of $f_1(H)$ and the critical field $H_{\mathrm{M}}$, after which the deviation from the $T(H^2)$ behavior sets in, are shown in Fig.S 3(b). In the case of Mott VRH regime [4], it is expected that $H_{\mathrm{M}} \sim T^{3/8} = T^{0.375}$, as highlighted in Fig.S 3(b) for comparison. Here, for GaN $H_{\mathrm{M}}$ varies as $T^{0.338}$, confirming that the observed NMR is due to Mott VRH in accord with $\rho(\mathrm{T})$ below 50 K.

The MR as a function of applied field for Sample B is depicted in Fig.S 3(c). The MR is positive with a $H^2$-dependence down to 150 K. Below 100 K the behavior of the MR indicates that the conduction is of the VRH Mott type, as described in the main text. This response is attributed to the presence of the GaN capping layer

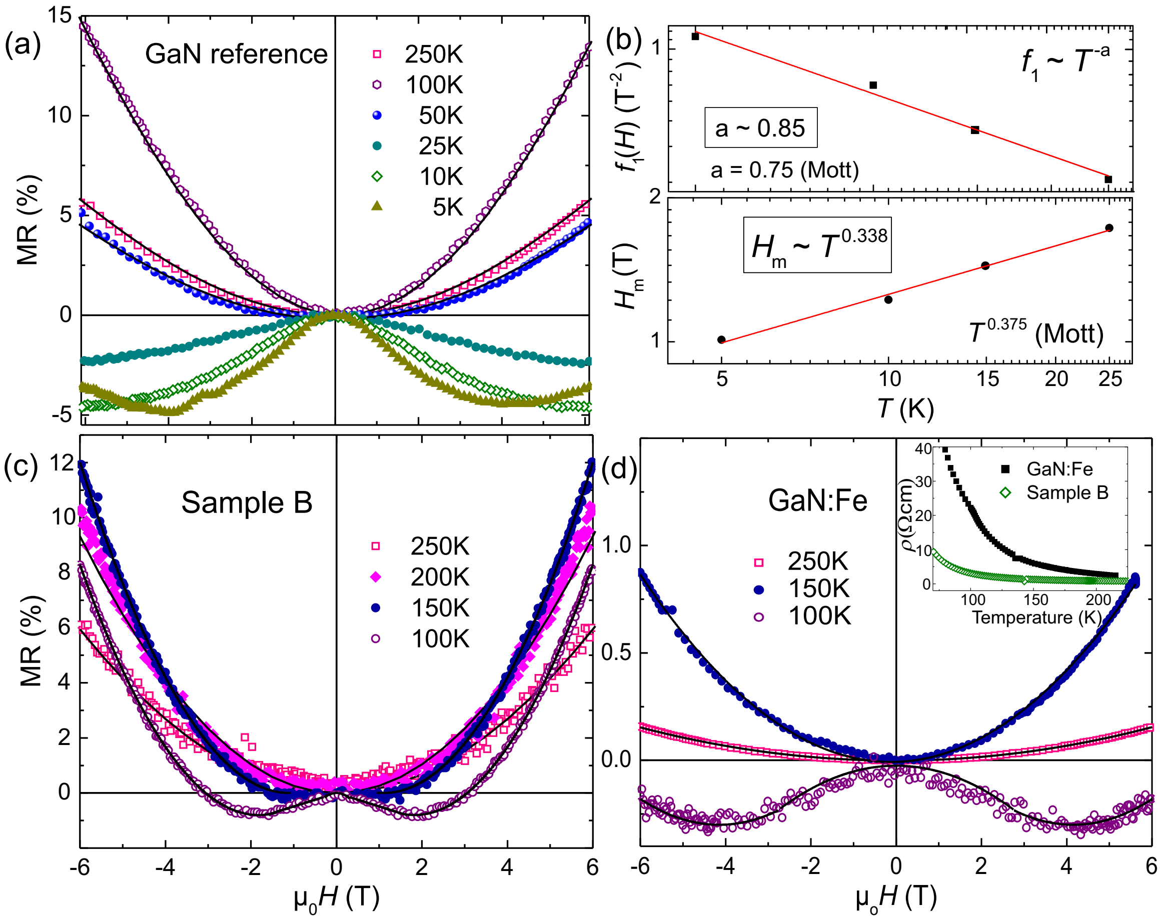


Fig.S 3: (a) Magnetoresistance curves as a function of applied magnetic field at different temperatures for the reference GaN sample. (b) Results of the analysis of the NMR observed at low temperatures in the low field region ($H<2\,\mathrm{T}$), pointing to a Mott VRH conduction below 50 K. Motts VRH regime: $H_{\mathrm{M}}\approx T^{0.375}$(c) MR as a function of applied magnetic field for Sample B acquired at different temperatures, and (d) of a dilute GaN:Fe layer grown on GaN. Inset to (d): resistivity *vs.* temperature of Sample B and of the GaN:Fe sample.

in Sample B and to the consequent increased disorder and diffusion of dilute Fe towards the sample surface. For confirmation, a 130 nm thick GaN:Fe layer grown on GaN is analysed and a similar behavior is observed, as shown in Fig.S 3(d), where the onset of the Arrhenius to Mott VRH is also observed at 100 K. The MR in this sample is 10 times lower than in Sample B, while the overall sample resisitivity is 5 times higher.

# References

[1] D. Zhang, K. J. Klabunde, C. M. Sorensen, and G. C. Hadjipanayis. Magnetization temperature dependence in iron nanoparticles. *Phys. Rev. B*, 58:14167, 1998.

[2] R. Abdia, A.El. Kaaouachi, A. Nafidi, G. Biskupski, and J. Hemine. Variable range hopping conductivity and negative magnetoresistance in $n$-type InP semiconductor. *Solid State Electron.*, 53:469–472, 2009.

[3] V.I. Nguyen, B.Z. Spivak, and B.I. Schklovskii. Aaronov-Bohm oscillations with normal and superconducting flux quanta in hopping conductivity. *JETP Lett.*, 41:42, 1985.

[4] N.F. Mott. *J. Non-Cryst. Solids*, 1:1, 1968.
